# Supplementary material for: Brownian systems with spatially inhomogeneous activity
Source: arXiv:1705.01392 source file (2017-05-03)
Supplement: Supplementary file 1 [file supplementary.pdf]

## Supplementary Information

### Rotational correlation

The equilibrium time-correlation function of a single, rotationally diffusing unit vector is defined according to the dyadic product

$$\langle \boldsymbol{p}(t)\boldsymbol{p}(t_0)\rangle = \int d\boldsymbol{p} \int d\boldsymbol{p}_0 \, \boldsymbol{p}\,\boldsymbol{p}_0 P_{\mathrm{r}}(\boldsymbol{p}, t\,|\,\boldsymbol{p}_0, t_0) P_{\mathrm{r}}^{\mathrm{eq}}(\boldsymbol{p}_0) \tag{S1}$$

where $P_{\mathrm{r}}(\boldsymbol{p}, t\,|\,\boldsymbol{p}_0, t_0)$ is the conditional probability of finding the vector $\boldsymbol{p}$ at time $t$, given that it was equal to $\boldsymbol{p}_0$ at earlier time $t_0$. We assume that the system was in equilibrium at $t_0$ with orientational distribution $P_{\mathrm{r}}^{\mathrm{eq}}(\boldsymbol{p}_0) = (4\pi)^{-1}$.

The conditional probability evolves in time according to the following time-evolution equation [1]

$$\frac{\partial}{\partial t} P_{\mathrm{r}}(\boldsymbol{p}, t\,|\,\boldsymbol{p}_0, t_0) = \Omega_{\mathrm{r}} P_{\mathrm{r}}(\boldsymbol{p}, t\,|\,\boldsymbol{p}_0, t_0) \tag{S2}$$

where $\Omega_{\mathrm{r}}$ is the rotational diffusion (Laplace-Beltrami) operator, given explicitly in spherical coordinates by

$$\Omega_{\mathrm{r}} = D_{\mathrm{r}} \left( \frac{1}{\sin(\theta)} \frac{\partial}{\partial \theta} \left( \sin(\theta) \frac{\partial}{\partial \theta} \right) + \frac{1}{\sin^2(\theta)} \frac{\partial^2}{\partial \phi^2} \right), \tag{S3}$$

where $D_{\mathrm{r}}$ is the rotational diffusion constant. Equation (S2) has the formal solution

$$P_{\mathrm{r}}(\boldsymbol{p}, t\,|\,\boldsymbol{p}_0, t_0) = e^{\Omega_{\mathrm{r}}(t-t_0)} \delta(\boldsymbol{p} - \boldsymbol{p}_0), \tag{S4}$$

for the initial condition $P_{\mathrm{r}}(\boldsymbol{p}, t_0\,|\,\boldsymbol{p}_0, t_0) = \delta(\boldsymbol{p} - \boldsymbol{p}_0)$. In the following it is important to note that $\Omega_{\mathrm{r}}$ in Eqs. (S2) and (S4) acts upon the orientation vector $\boldsymbol{p}$ and not on the initial value $\boldsymbol{p}_0$.

Substitution of (S4) into (S1) yields

$$\langle \boldsymbol{p}(t)\boldsymbol{p}(t_0)\rangle = \int d\boldsymbol{p} \int d\boldsymbol{p}_0 \, P_{\mathrm{r}}^{\mathrm{eq}}(\boldsymbol{p}_0)\, \boldsymbol{p}\,\boldsymbol{p}_0\, e^{\Omega_{\mathrm{r}}(t-t_0)} \delta(\boldsymbol{p} - \boldsymbol{p}_0). \tag{S5}$$

By introducing the adjoint operator, $\Omega_{\mathrm{r}}^{\dagger}$, the delta function can be brought to the front of the integrand

$$\langle \boldsymbol{p}(t)\boldsymbol{p}(t_0)\rangle = \int d\boldsymbol{p} \int d\boldsymbol{p}_0 \, \delta(\boldsymbol{p} - \boldsymbol{p}_0) P_{\mathrm{r}}^{\mathrm{eq}}(\boldsymbol{p}_0)\, \boldsymbol{p}_0 e^{\Omega_{\mathrm{r}}^{\dagger}(t-t_0)} \boldsymbol{p}, \tag{S6}$$

where we have used the fact that $\boldsymbol{p}_0$ commutes with the propagator. As the rotational diffusion operator is self-adjoint we have that $\Omega_{\rm r}^\dagger = \Omega_{\rm r}$. Using the delta function to evaluate the integral over $\boldsymbol{p}_0$ yields

$$\begin{aligned}\langle \boldsymbol{p}(t)\boldsymbol{p}(t_0)\rangle &= \int d\boldsymbol{p}\, P_{\rm r}^{\rm eq}(\boldsymbol{p})\, \boldsymbol{p}\, e^{\Omega_{\rm r}^\dagger (t-t_0)}\, \boldsymbol{p}, \\ &= \langle\, \boldsymbol{p}\, e^{\Omega_{\rm r}^\dagger (t-t_0)}\, \boldsymbol{p}\, \rangle_{\rm r,eq} \end{aligned} \tag{S7}$$

where $\langle \cdot \rangle_{\rm r,eq}$ indicates an equilibrium average over the orientational distribution. One thus arrives at the interpretation that the propagator $e^{\Omega_{\rm r}^\dagger (t-t_0)}$ evolves the orientation vector, according to the diffusional dynamics of Eq. (S3), from $t_0$ to the later time $t$. The correlation function is then obtained by averaging over the initial, equilibrium distribution function.

In order to obtain an explicit expression for the correlation function (S7) we return to Eq. (S2). By expanding the conditional distribution function in spherical harmonics (the eigenfunctions of $\Omega_{\rm r}$) it can readily be shown that the general solution of (S2) is given by [2]

$$P_{\rm r}(\boldsymbol{p}, t\,|\,\boldsymbol{p}_0, t_0) = \sum_{l=0}^{\infty} \sum_{m=-l}^{l} e^{-D_r l(l+1)(t-t_0)} Y_{lm}^*(\theta_0, \phi_0) Y_{lm}(\theta, \phi), \tag{S8}$$

where $Y_{lm}$ is a spherical harmonic. Substitution of (S8) into (S1) and expression of the unit vectors in spherical coordinates, $\boldsymbol{p} = (\cos\phi \sin\theta, \sin\phi \sin\theta, \cos\theta)$, then yields the desired result

$$\langle\, \boldsymbol{p}\, e^{\Omega_{\rm r}^\dagger (t-t_0)}\, \boldsymbol{p}\, \rangle_{\rm r,eq} = \frac{\mathbf{1}}{3} e^{-2D_{\rm r}(t-t_0)}, \tag{S9}$$

where $\mathbf{1}$ is the unit tensor. If the correlation is required between particle labelled unit vectors (e.g. between $\boldsymbol{p}_i$ and $\boldsymbol{p}_j$), then the result (S9) is supplemented by a Kronecker-delta factor, $\delta_{ij}$, because the rotational diffusion of distinct particles is uncorrelated for the model system of interest.

### Large activity parameters

We have not made a systematic study of the range of validity of the linear response. With three parameters $v_a$, $\omega$, and $\rho_b$, it is a difficult task to identify the range over which the linear response is accurate and will be pursued in future. Here we present few particular cases where the linear reponse is clearly insufficient to describe the average orientation. In Fig. S1 we show the average orientation for large values of activity, $v_a = 40$ and 60, for

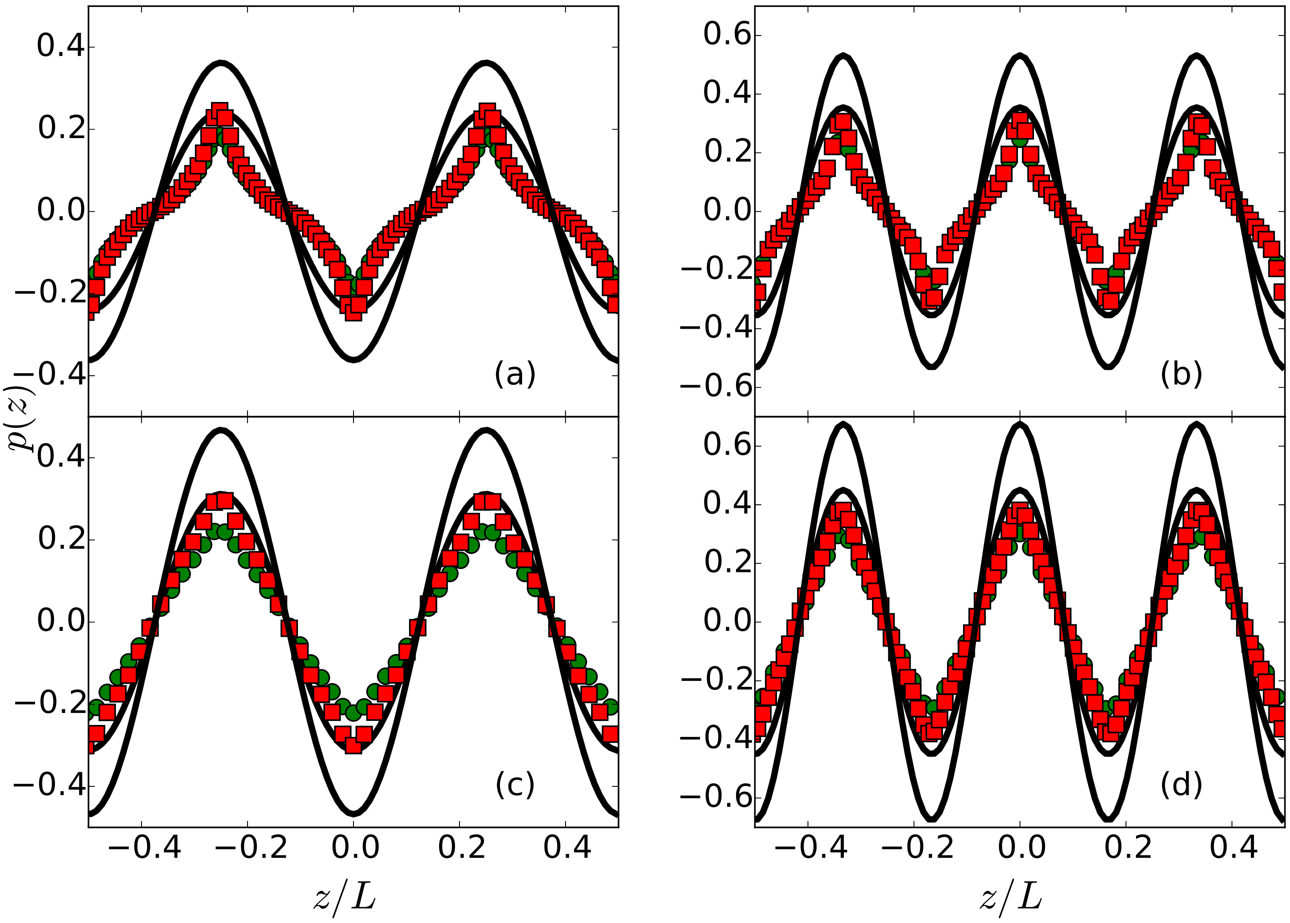


**Supplementary Figure** S1. Average orientation per particle in the $\hat{\boldsymbol{e}}_z$ direction for $\rho_b = 0.2$ in (a) and (b) and $\rho_b = 0.6$ in (c) and (d). The activity field is $v_0(z) = v_a \sin(\omega(z + 0.5L))$ with the angular frequency $\omega = n\omega_0$, where $\omega_0 = 2\pi/L$ and $n$ is a parameter. In (a) and (c), $\omega = 2\omega_0$ whereas in (b) and (d), $\omega = 3\omega_0$. The circles correspond to $v_a = 40$ and the squares to $v_a = 60$. The thick lines corresond to the theoretical prediction of Eq. (20) in the main text. For the parameters considered here, the theory significantly overestimates the average orientation. There are clear signatures of nonlinearity in (a) and (b). This is to be expected as the linear order result of Eq. (20) is not valid for large values of the activity-parameters.

low density $\rho_b = 0.2$ and high density $\rho_b = 0.6$. For such large values of activity, the theoretical prediction significantly overestimates the average orientation. For low density, the large activity introduces higher-order harmonics in the average orientation as can be seen in Fig. S1(a,b). These higher-order harmonics do not feature as prominently for the

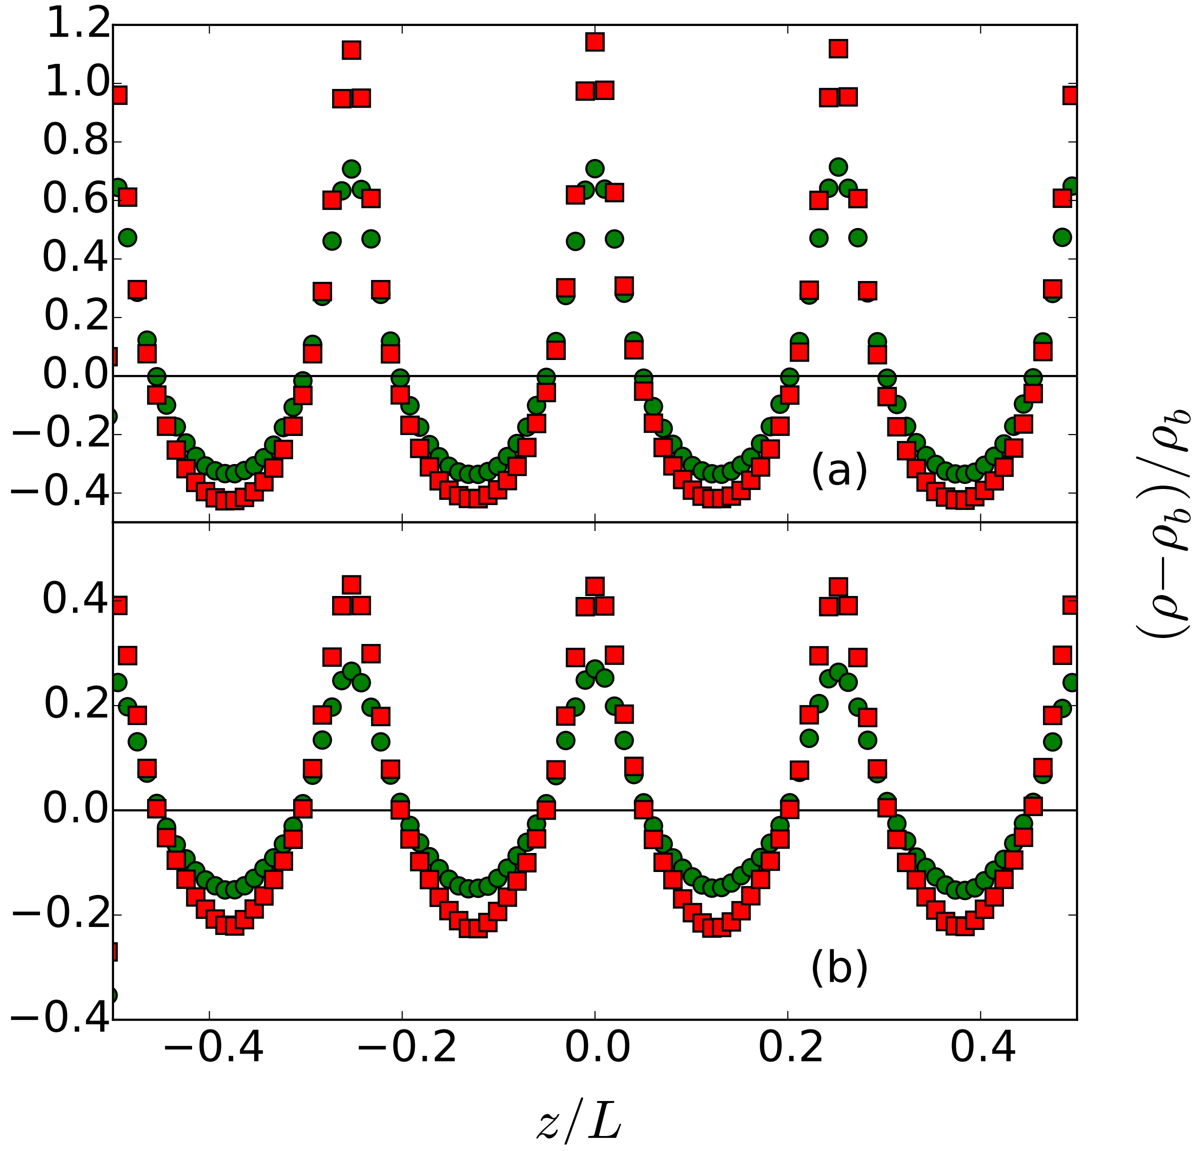


**Supplementary Figure** S2. Relative change in density $(\rho-\rho_b)/\rho_b$ for $\rho_b = 0.2$ in (a) and $\rho_b = 0.6$ in (b) for sinusoidal activity with $\omega = 2\omega_0$. The circles correspond to $v_a = 40$ and the squares to $v_a = 60$. Particles accumulates at the nodes of the activity and the change in density is asymmetric. The density more than doubles at the nodes of the activity in (a) for $v_a = 60$.

high density case as can be seen in Fig. S1(c,d).

Nonlinearities are also evident in the density profiles as shown in Fig. S2. For large activity, there is a large change in the density for $\rho_b = 0.2$ exceeding 100% at the nodes of the activity for $v_a = 60$. It is therefore expected that for such large activity, there are large

nonlinear deviations present in the average orientation. For the bulk density $\rho_b = 0.6$, the change in density due to the activity is smaller than that in the case of $\rho_b = 0.2$, however, it is still large in absolute terms such that our linear response formula for the average orientation, based on the assumption of uniform density, is certainly invalid.

## References


[1] H. Risken, *The Fokker-Planck equation* (Springer, Berlin, 1989).

[2] T. F. Farage, P. Krinninger, and J. M. Brader, Physical Review E **91**, 042310 (2015).
